# Supplementary material for: Optical line shapes of color centers in solids from classical autocorrelation functions
Source: arXiv:2408.06908 ancillary file (2024-08-13)
Supplement: Supplementary file 1 [file supporting-information.pdf]

Supporting Information

# Optical line shapes of color centers in solids from classical autocorrelation functions

Christopher Linderälv,[1,2] Nicklas Österbacka,[1] Julia Wiktor,[1] and Paul Erhart[1,*]

[1] Department of Physics, Chalmers University of Technology, SE-41296, Gothenburg, Sweden

[2] University of Oslo, Department of Physics, Centre for Material Science and Nanotechnology, P.O. Box 1048, Blindern, Oslo N-0316, Norway

[*] erhart@chalmers.se

# Contents

**Supplementary Notes** **1**
S1. Density functional theory calculations . . . 1
S2. Construction of the machine-learned potential . . . 1
S3. Molecular dynamics and auto-correlation functions . . . 2
S4. Effect of choice of prefactor . . . 2

**Supplementary Figures** **2**
S1. Orbitals of the $(V_{Si}V_C)^0_{kk}$ defect in the ground state . . . 2
S2. Orbitals of the $(V_{Si}V_C)^0_{kk}$ defect in the excited state . . . 3
S3. Parity plots for the machine-learned potential . . . 3
S4. Effect of broadening and prefactor on the spectral density . . . 3

**Supplementary References** **4**

# Supplementary Notes

## Supplementary Note S1: Density functional theory calculations

Collinear spin-polarized density functional theory (DFT) calculations were performed using the projector augmented wave method [1, 2] as implemented in the Vienna ab-initio simulation package [3–5] with a plane wave energy cutoff of 520 eV and the PBEsol exchange-correlation functional [6]. The Brillouin zone was sampled with automatically generated Γ-centered $\boldsymbol{k}$-point grids with a maximum spacing of $0.25\,\text{Å}^{-1}$. The excited state was obtained by enforcing the occupation of the first defect level in the $\beta$-spin channel to zero ($\beta$, $n = 1$ in Figure S2) and the occupation of the second level to one ($\beta$, $n = 2$ in Figure S2) as in Ref. 7.

## Supplementary Note S2: Construction of the machine-learned potential

We constructed a machine-learning potential (MLP) model using the neuroevolution potential (NEP) framework [8–10] and the iterative strategy outlined in Ref. 11 utilizing the GPUMD [10] and CALORINE packages [12]. Training structures included configurations along the configuration coordinate (Figure 2d) as well as snapshots from molecular dynamics (MD) simulations (see below) of ideal and defective structures at a range of system sizes. The MD structures were generated via an active learning strategy and randomly selected from MD trajectories run at temperatures between 70 and 400 K and at pressures ranging from −2.5 to 10 GPa. In total the training set consisted of 1341 structures, corresponding to a total of 448 388 atoms, including 59 defect-free as well as 641 structures each of defect structures on the ground and excited state potential energy surfaces (PESs). Structure generation and manipulation were carried out using the ASE [13] and HIPHIVE packages [14].

The final NEP model was obtained after 3 iterations and trained using all available reference data. In addition we trained an ensemble model using five folds to estimate the model error via $k$-fold cross validation. The resulting root mean square errors (RMSEs) are $(0.170 \pm 0.004)\,\text{meV atom}^{-1}$ for the energies and (32.1 ±

0.8) meV Å$^{-1}$ for the forces. The corresponding average coefficients of determination on the same folds are $R^2 = 0.999\,980 \pm 0.000\,006$ and $R^2 = 0.998\,00 \pm 0.000\,03$ for energies and forces, respectively (Figure S3).

Phonon dispersions for the ideal structure (Figure 3b) were obtained using forces from DFT calculations and NEP model using a $6 \times 6 \times 2$ supercell and the PHONOPY package [15].

The reference data obtained through DFT calculations is available in the form of ASE sqlite databases on zenodo at `https://doi.org/10.5281/zenodo.13284738`. The record also includes the NEP model in a format suitable for the GPUMD package.

## Supplementary Note S3: Molecular dynamics and auto-correlation functions

To sample the autocorrelation function (ACF) in Eq. (11) of the main paper, we employed supercells comprising $74 \times 74 \times 23$ primitive unit cell, corresponding to 1 007 582 atoms in the defect configurations. For each temperature we carried out simulations using 50 different initial configurations that were obtained by NVT simulations at the 0 K lattice parameters as predicted by the NEP model, i.e., $a = 3.080$ Å and $c = 10.082$ Å. For each of these a MD simulation in the NVE ensemble was conducted for 40 ps. The ACF was evaluated up to a time lag of 12 ps. Furthermore, in computing the average of Eq. (11), the time was reset to zero every 0.5 ps. In total, the average of the ACF was computed over 1500 trajectories. The damping was effectively zero for the very large systems due to natural decay of the ACF. The lower frequency cutoff for evaluation of $F(\omega)$ was 5 meV to avoid amplifying low energy noise by dividing with very small numbers.

## Supplementary Note S4: Effect of choice of prefactor

Since the sampling here is done using classical MD simulations the phonon mode occupations follow classical statistics, yielding the classical ACF, Eq. (11). The transition from the classical to the quantum ACF is approximated via Eq. (13), which involves the choice of the prefactor $f(\beta\omega)$. Here, in line with earlier work [16] we chose the harmonic prefactor $f(\beta\omega) = \beta\omega/2$, rather than the so-called standard prefactor $\tanh(\beta\omega/2)$ [17].

When using the harmonic prefactor the main peak of the spectral density function at around 30 meV exhibits a weak temperature dependence while at higher energies ($\geq 60$ meV) the spectral density is almost temperature independent (Figs. 5 and S4c). By contrast when using the standard prefactor, the temperature dependence is significant for all energies (Figure S4d). This prefactor saturates at unity for $\beta\omega/2 \gtrsim 2$, and thus has little effect for phonon with energies above 50 meV for the 70 K and 150 K spectral densities.

The good agreement with reference optical emission spectra as well as the consistency between the Stokes shifts computed using static configurations and the spectral distribution function, show, however, the harmonic prefactor ($f(\beta\omega) = \beta\omega/2$) to be the suitable choice for the present system. The latter balances the classical ACF to make it almost fully temperature independent. This implies that the temperature dependence of the spectral density (Figure S4c) and emission line shape (Figure 6a) originate from other parts of the cumulant rather than from the spectral density.

# Supplementary Figures

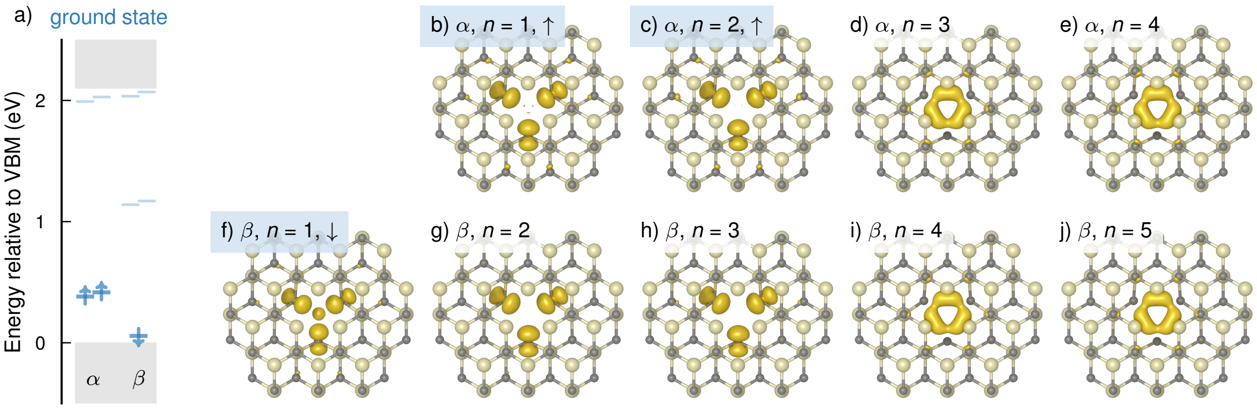


**Fig. S1: Orbitals of the $(V_{Si}V_C)^0_{kk}$ defect in the ground state.** (a) Defect level structure and (b–j) corresponding orbitals superimposed on the defect configuration. The orbitals are indexed from lowest to highest energy starting at $n = 1$ for each spin channel. Occupied orbitals are highlighted in blue in (b–j).

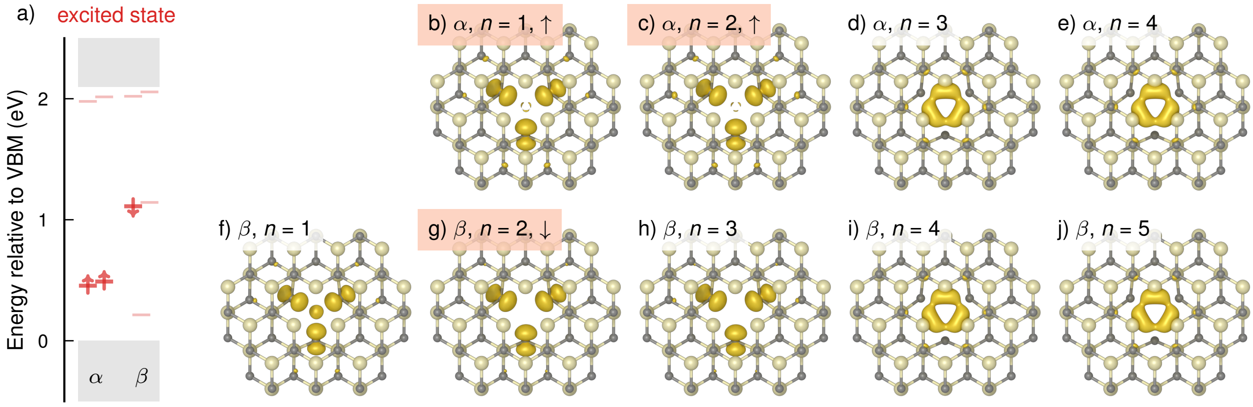


**Fig. S2: Orbitals of the $(\mathrm{V_{Si}V_C})^0_{kk}$ defect in the excited state.** (a) Defect level structure and (b–j) corresponding orbitals superimposed on the defect configuration. The orbitals are indexed from lowest to highest energy starting at $n = 1$ for each spin channel. Occupied orbitals are highlighted in red in (b–j).

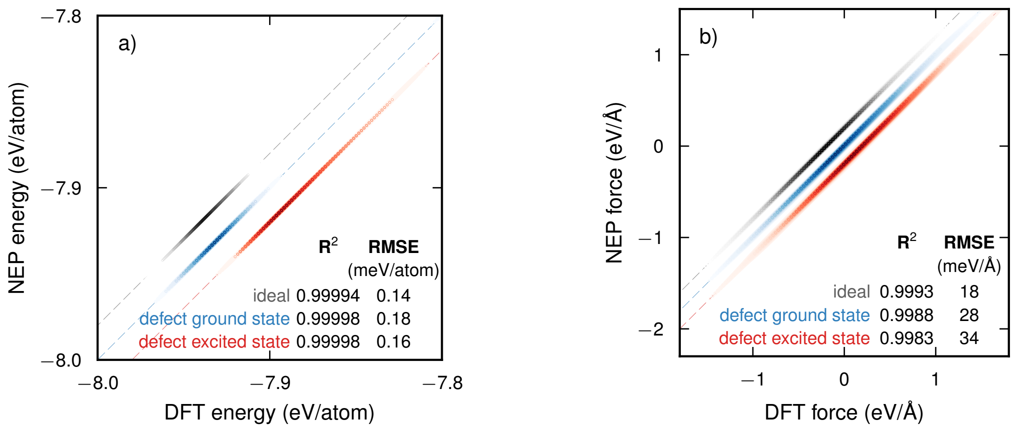


**Fig. S3: Parity plots for the machine-learned potential.** The data for (a) energy and (b) forces are presented in the form of kernel density estimates comparing results from the NEP model with DFT reference data. Coefficients of determination ($R^2$) and root mean square error (RMSE) for subsets of the data are shown in the tables.

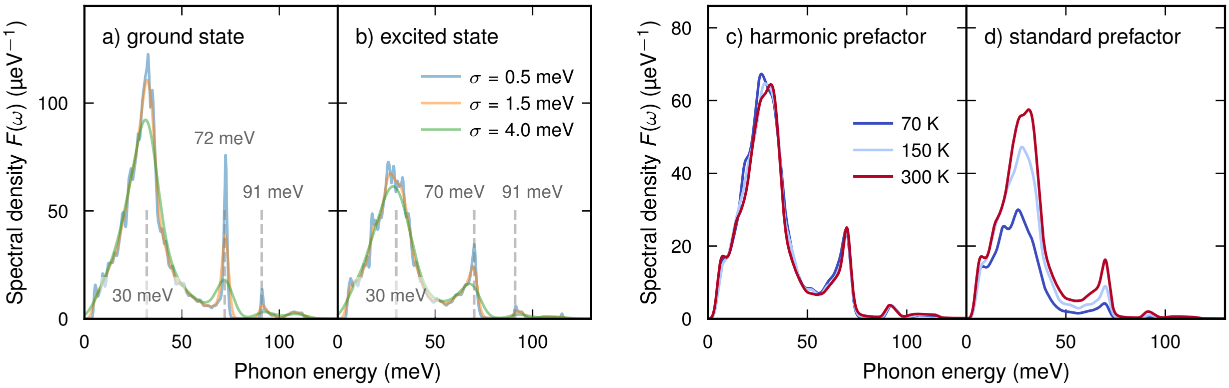


**Fig. S4: Effect of broadening and prefactor on the spectral density.** (a, b) Spectral densities at 70 K using different levels of broadening. (c, d) Effect of the prefactor $f(\beta\omega)$, see Eq. (13) in the main paper, included for treating quantum effects on the spectral density.

# Supplementary References


[1] P. E. Blöchl, *Projector augmented-wave method,* Physical Review B **50**, 17953 (1994). doi:10.1103/PhysRevB.50.17953.

[2] G. Kresse and D. Joubert, *From ultrasoft pseudopotentials to the projector augmented-wave method,* Physical Review B **59**, 1758 (1999). doi:10.1103/PhysRevB.59.1758.

[3] G. Kresse and J. Hafner, *Ab initio molecular dynamics for liquid metals,* Physical Review B **47**, 558 (1993). doi:10.1103/PhysRevB.47.558.

[4] G. Kresse and J. Furthmüller, *Efficient iterative schemes for ab initio total-energy calculations using a plane-wave basis set,* Physical Review B **54**, 11169 (1996). doi:10.1103/PhysRevB.54.11169.

[5] G. Kresse and J. Furthmüller, *Efficiency of ab-initio total energy calculations for metals and semiconductors using a plane-wave basis set,* Computational Materials Science **6**, 15 (1996). doi:https://doi.org/10.1016/0927-0256(96)00008-0.

[6] J. P. Perdew, A. Ruzsinszky, G. I. Csonka, O. A. Vydrov, G. E. Scuseria, L. A. Constantin, X. Zhou, and K. Burke, *Restoring the Density-Gradient Expansion for Exchange in Solids and Surfaces,* Physical Review Letters **100**, 136406 (2008). doi:10.1103/PhysRevLett.100.136406.

[7] Y. Jin, M. Govoni, G. Wolfowicz, S. E. Sullivan, F. J. Heremans, D. D. Awschalom, and G. Galli, *Photoluminescence spectra of point defects in semiconductors: Validation of first-principles calculations,* Physical Review Materials **5**, 084603 (2021). doi:10.1103/PhysRevMaterials.5.084603.

[8] Z. Fan, Z. Zeng, C. Zhang, Y. Wang, K. Song, H. Dong, Y. Chen, and T. Ala-Nissila, *Neuroevolution machine learning potentials: Combining high accuracy and low cost in atomistic simulations and application to heat transport,* Physical Review B **104**, 104309 (2021). doi:10.1103/PhysRevB.104.104309.

[9] Z. Fan, *Improving the accuracy of the neuroevolution machine learning potential for multi-component systems,* Journal of Physics: Condensed Matter **34**, 125902 (2022). doi:10.1088/1361-648x/ac462b.

[10] Z. Fan, Y. Wang, P. Ying, K. Song, J. Wang, Y. Wang, Z. Zeng, K. Xu, E. Lindgren, J. M. Rahm, A. J. Gabourie, J. Liu, H. Dong, J. Wu, Y. Chen, Z. Zhong, J. Sun, P. Erhart, Y. Su, and T. Ala-Nissila, *GPUMD: A Package for Constructing Accurate Machine-Learned Potentials and Performing Highly Efficient Atomistic Simulations,* The Journal of Chemical Physics **157**, 114801 (2022). doi:10.1063/5.0106617.

[11] E. Fransson, J. Wiktor, and P. Erhart, *Phase Transitions in Inorganic Halide Perovskites from Machine-Learned Potentials,* The Journal of Physical Chemistry C **127**, 13773 (2023). doi:10.1021/acs.jpcc.3c01542.

[12] E. Lindgren, M. Rahm, E. Fransson, F. Eriksson, N. Österbacka, Z. Fan, and P. Erhart, *calorine: A Python package for constructing and sampling neuroevolution potential models,* Journal of Open Source Software **9**, 6264 (2024). doi:10.21105/joss.06264.

[13] A. H. Larsen, J. J. Mortensen, J. Blomqvist, I. E. Castelli, R. Christensen, M. Duak, J. Friis, M. N. Groves, B. Hammer, C. Hargus, E. D. Hermes, P. C. Jennings, P. B. Jensen, J. Kermode, J. R. Kitchin, E. L. Kolsbjerg, J. Kubal, K. Kaasbjerg, S. Lysgaard, J. B. Maronsson, T. Maxson, T. Olsen, L. Pastewka, A. Peterson, C. Rostgaard, J. Schiøtz, O. Schütt, M. Strange, K. S. Thygesen, T. Vegge, L. Vilhelmsen, M. Walter, Z. Zeng, and K. W. Jacobsen, *The atomic simulation environmenta Python library for working with atoms,* Journal of Physics: Condensed Matter **29**, 273002 (2017). doi:10.1088/1361-648X/aa680e.

[14] F. Eriksson, E. Fransson, and P. Erhart, *The Hiphive Package for the Extraction of High-Order Force Constants by Machine Learning,* Advanced Theory and Simulations **2**, 1800184 (2019). doi:10.1002/adts.201800184.

[15] A. Togo, *First-principles Phonon Calculations with Phonopy and Phono3py,* Journal of the Physical Society of Japan **92**, 012001 (2023). doi:10.7566/JPSJ.92.012001.

[16] S. Valleau, A. Eisfeld, and A. Aspuru-Guzik, *On the alternatives for bath correlators and spectral densities from mixed quantum-classical simulations,* The Journal of Chemical Physics **137**, 224103 (2012). doi:10.1063/1.4769079.

[17] S. A. Egorov, K. F. Everitt, and J. L. Skinner, *Quantum Dynamics and Vibrational Relaxation,* The Journal of Physical Chemistry A **103**, 9494 (1999). doi:10.1021/jp9919314.
